# Supplementary material for: Foreground removal and 21 cm signal estimates: comparing different blind methods for the BINGO Telescope
Source: arXiv:2209.11701 source file (2026-02-05)
Supplement: Supplementary file 1 [file AppendixC_rec.tex]

The accuracy of the \HI\ reconstruction depends on several factors, including the number and type of foreground components, the instrumental noise model, the beam shape, map resolution, sidelobe contamination, polarization leakage, frequency channel, signal-to-noise ratio, the foreground-removal algorithm, and the number of simulations used in the noise-debiasing procedure.

In this work, we assumed a common angular resolution of 40 arcmin with a Gaussian beam, five foreground components, white noise only (no $1/f$ noise), and no polarization leakage or sidelobe effects. We considered three foreground-removal methods and up to 400 simulations for the debiasing step.

We illustrate the reconstruction obtained with 400 realizations for four representative channels (1st, 10th, 20th, and 30th) in Figs.~\ref{fig: recGMCA} (GMCA), \ref{fig: recGNILC} (GNILC), and \ref{fig: recFastICA} (FastICA). For GMCA and FastICA we use $n_{\mathrm{s}}=3$ templates.

\begin{figure}
\centering
    \includegraphics[width=0.49\textwidth]{images/GMCA_bin0.jpg}
    \includegraphics[width=0.49\textwidth]{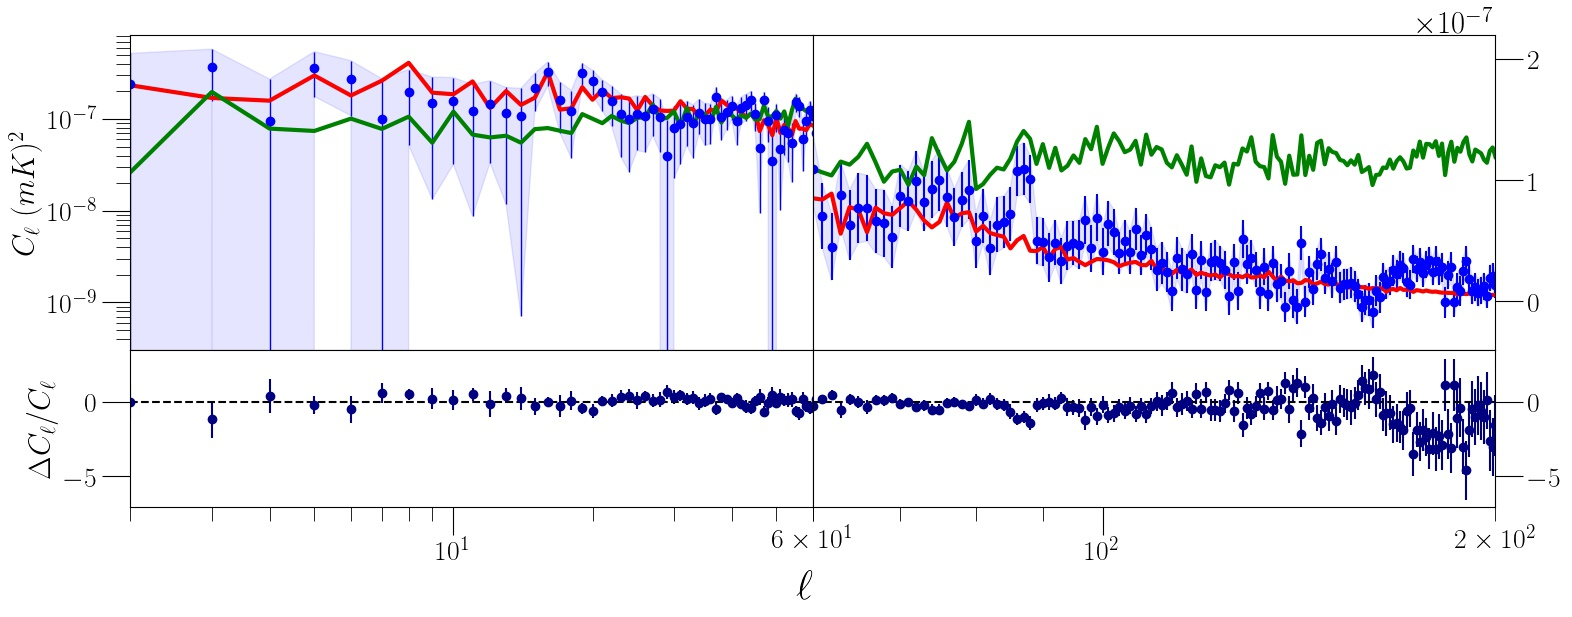}\\
    \includegraphics[width=0.49\textwidth]{images/GMCA_bin19.jpg}
    \includegraphics[width=0.49\textwidth]{images/GMCA_bin29.jpg}
\caption{Reconstructed \HI\ angular power spectra for the 1st (top left), 10th (top right), 20th (bottom left), and 30th (bottom right) channels using GMCA with 400 realizations and $n_{\mathrm{s}}=3$. The blue curve shows the reconstructed \HI, the red curve the input \HI, and the green curve the white-noise spectrum. Below each panel we show the residual difference between reconstructed and input \HI\ spectra.}
\label{fig: recGMCA}
\end{figure}

\begin{figure}
\centering
    \includegraphics[width=0.49\textwidth]{images/GNILC_bin0.jpg}
    \includegraphics[width=0.49\textwidth]{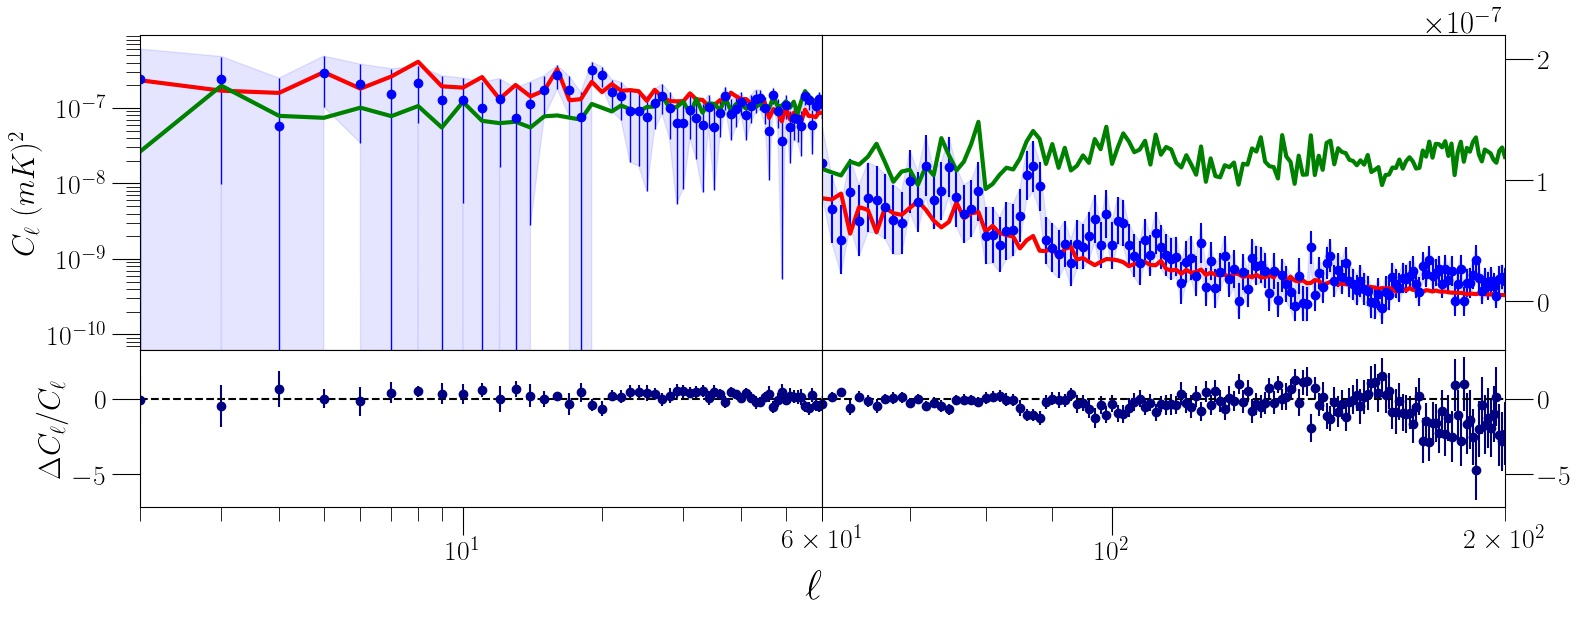}\\
    \includegraphics[width=0.49\textwidth]{images/GNILC_bin19.jpg}
    \includegraphics[width=0.49\textwidth]{images/GNILC_bin29.jpg}
\caption{Same as Fig.~\ref{fig:recGMCA}, but using GNILC with 400 realizations.}
\label{fig: recGNILC}
\end{figure}

\begin{figure}
\centering
    \includegraphics[width=0.49\textwidth]{images/ICA_bin0.jpg}
    \includegraphics[width=0.49\textwidth]{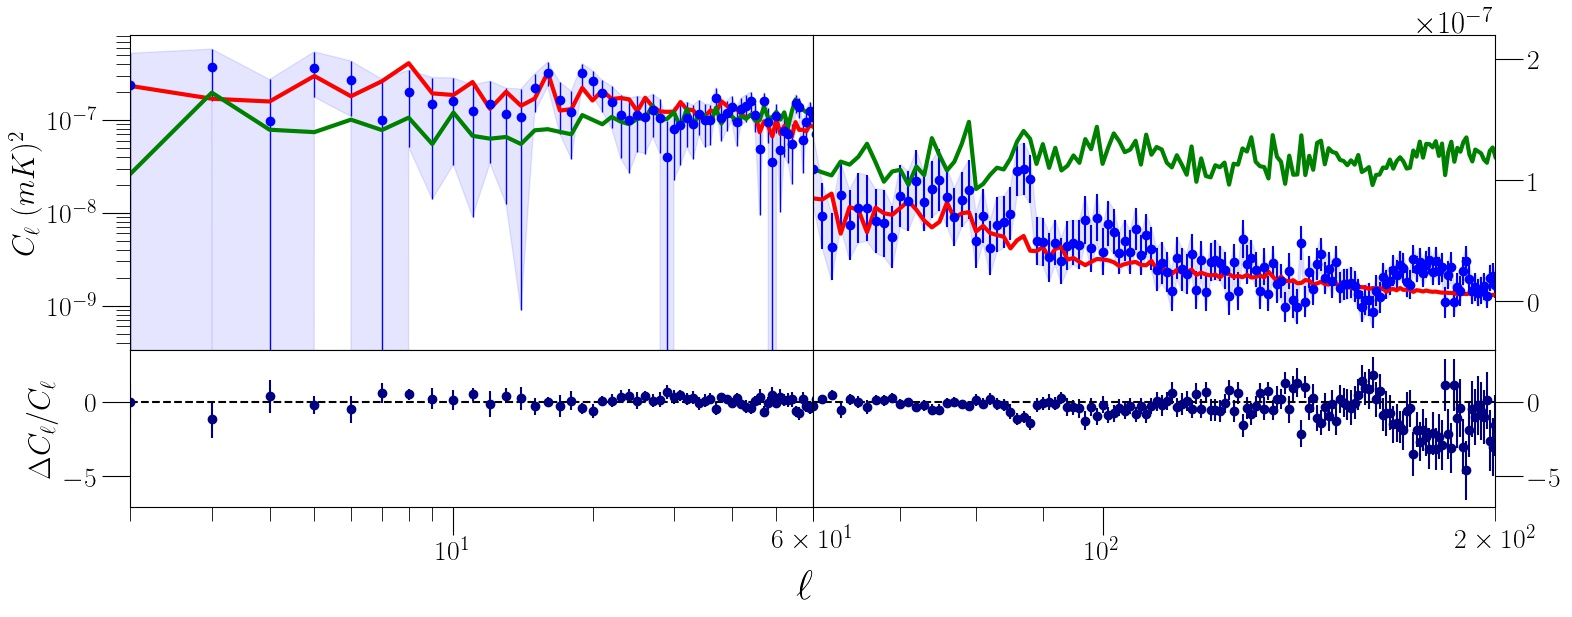}\\
    \includegraphics[width=0.49\textwidth]{images/ICA_bin19.jpg}
    \includegraphics[width=0.49\textwidth]{images/ICA_bin29.jpg}
\caption{Same as Fig.~\ref{fig:recGMCA}, but using FastICA with 400 realizations and $n_{\mathrm{s}}=3$.}
\label{fig: recFastICA}
\end{figure}
